# Supplementary material for: Ego2X: Contact-aware Transfer from Egocentric Human Data to Any Robot
Source: arXiv:2611.24138 source file (2026-11-19)
Supplement: Supplementary file 1 [file X_suppl.tex]

\clearpage
\hypersetup{pageanchor=false}
\setcounter{page}{1}
\maketitlesupplementary
\appendix

\section{Evaluation Protocol and Statistical Disclosures}
\label{sec:supp-protocol}

\begin{table}[t]
\centering
\scriptsize
\renewcommand{\arraystretch}{0.95}
\setlength{\tabcolsep}{2.5pt}
\caption{\textbf{Notation, evaluation subsets, and pipeline shorthand} used across the main paper and supplementary material.}
\label{tab:suppl_notation}
\begin{tabular*}{\columnwidth}{@{\extracolsep{\fill}}p{0.27\columnwidth}p{0.68\columnwidth}@{}}
\toprule
Symbol / Term & Definition \\
\midrule
$\phi_o$ & Exact non-convex object signed distance field (SDF). \\
$\mathbf{T}_{WO}^t, \mathbf{T}_{WG}^t, \mathbf{T}_{OG}$ & World-object, world-gripper, and locked object-frame grasp poses ($\mathrm{med}_3$: $3$-frame temporal median filter). \\
$\mathbf{c}_{t,k}$ & Object-centric CORE record $(\mathbf{p}_{t,k},\mathbf{f}_{t,k},m_{t,k},s_{t,k})$ per frame $t$ and link $k$ (anchor, force prior, mode, state). \\
$\rho_{t,k},\, f^{\mathrm{lb}}_{t,k}$ & Normalized part-load share and kinematic support-load lower-bound prior. \\
\midrule
\texttt{LOCO} & Leave-one-clip-out cross-validation ($36$-clip pool). \\
\texttt{ALL} / \texttt{GEOM} / $\texttt{GEOM}{\cap}\texttt{HC}$ & All $25{,}549$ EgoDex slots / geometrically supported ($\le 15\,\mathrm{mm}$ to $\phi_o$) / intersected with high-confidence EgoTac contacts. \\
\texttt{Band A} & True-mesh two-pad signed distance in $[-4.5,+5.5]\,\mathrm{mm}$. \\
\texttt{bPOA} & Balanced part-occlusion accuracy (mean of front-of-object and behind-object occlusion accuracy). \\
\midrule
\texttt{CARD} / \texttt{wf} & Contact-driven dexterous IK (Eq.~\ref{eq:ik}) / controlled wrist-following IK baseline. \\
\texttt{POSEVERIFY} & $29$-feature monotonic GBDT pose credibility scorer. \\
\texttt{B\_RAY\_FUSE} / \texttt{FUSE} & Contact-aligned object depth scale fusion (\texttt{CONF8} / \texttt{CONFIRM11}: $8$ confirmation / $11$ held-out clips). \\
\texttt{OW+M1lin} & Hand-ruler-free multi-view object triangulation with $15$-frame linear interval propagation. \\
\texttt{centroid clamping} & Clamping antipodal grasp midpoints toward the object support-hull centroid. \\
\texttt{zero-retry} & Episodes passing closed-loop simulator verification on the first attempt without planner retry. \\
\texttt{P70} / \texttt{55 lw} & All $70$ verified episodes / $55$ layout-weighted verified episodes. \\
\bottomrule
\end{tabular*}
\end{table}

\noindent\textbf{Splits and pre-registration.}
\Cref{tab:suppl_notation} summarizes our mathematical notation, evaluation subsets, and pipeline shorthand. HOT3D contact and dexterous IK evaluations use $31$ confirmation clips ($4{,}833$ ground-truth contact frames, $34$ unscoreable, $4{,}799$ scoreable; $92$ ground-truth intervals, $76$ matched by full CORE; $5{,}178$ state-scored frames). Stage-2 depth and pose credibility evaluations use disjoint development ($12$ clips; $36$-clip pool for out-of-fold \texttt{LOCO} training), confirmation ($8$ clips), held-out ($11$ clips), and fresh ($11$ clips) splits. Confirmatory hypotheses and evaluation scripts were locked prior to held-out testing. Cluster-bootstrap $95\%$ confidence intervals use $10{,}000$ resamples (seed $0$) over clips (HOT3D), parent takes or take-sides (EgoDex), and scene seeds (RoboTwin~2.0).

\noindent\textbf{Field-selective contact readout.}
CORE's native stage-specific (field-selective) readout operates with zero retraining and routes each exported field directly from its highest-precision evidence stage: contact intervals, frame masks, and tIoU read from $T{+}R{+}B$, grasp mode and interaction state read from $T{+}R{+}B{+}E$ (identical by construction), and 3D contact anchors read observed or rigidly carried $T{+}R$ ray hits with EgoTac surface fallback. On an independent $8$-clip held-out check, stage-specific readout lowers median contact-point error from $7.65$ to $3.84$\,mm ($\Delta=-3.80$\,mm, $95\%$ upper CI $-0.18$\,mm at $B=4\times 10^5$, $P(\Delta\ge 0)=0.024$, improving $7/8$ clips).

\noindent\textbf{Two-part contact force prior.}
Because monocular observations capture only visible hand-object facets, observed contact sets are wrench-incomplete on $75\%$ to $92.4\%$ of contact frames across manipulation takes. Rather than solving ill-posed Newton wrench balances for unique point forces, CORE exports a two-part contact force prior per link $k$: (i) normalized part-load shares $\rho_{t,k}$ distilled from EgoTac~\cite{egotac}, which achieve a $0.900$ median Spearman rank correlation with ground-truth contacting hand parts on HOT3D, and (ii) a hand-borne kinematic normal/support load lower-bound prior
\begin{equation}
f^{\mathrm{lb}}_{t,k} = m_{\mathrm{band}}\,\|\mathbf{a}_{\mathrm{COM},t}-\mathbf{g}\|\,w^{\mathrm{hand}}_t\,\rho_{t,k},
\end{equation}
computed with Gaussian temporal smoothing ($\sigma=1.0$) across canonical object density bands $\varrho_{\mathrm{band}}\in\{0.5,1.0,1.5\}\,\mathrm{g/mL}$. A closed-loop replay in Isaac Sim~\cite{isaaclab} confirms that simulated contact impulses align with exported CORE contact intervals and part-load priors under declared mass and friction parameters.

\noindent\textbf{Stage-2 depth and pose credibility analysis.}
The decoupled hand depth path (\texttt{OW+M1lin}, hand-ruler-free object triangulation with $15$-frame inner-edge linear interval propagation) was selected on the $12$-clip development split ($-2.60$\,mm $[-6.53,+2.79]$, valid/total coverage $98.5/75.9\%$; constant median propagation reaches $-4.17$\,mm on development vs.\ $-3.89$ and $-1.71$\,mm on the $8$-clip confirmation and $11$-clip held-out splits) and evaluated once on confirmation ($-4.31$\,mm $[-7.87,-1.38]$) and held-out ($-1.91$\,mm $[-4.53,-0.04]$) splits. On static-camera EgoDex videos ($\approx 1$\,mm/frame head motion, below the $15$\,mm parallax gate), all $81$ converted episodes abstain cleanly ($\delta\equiv 0$). On the $11$-clip held-out split, contact-aligned object depth fusion (\texttt{FUSE}) lowers in-contact object translation error from $141.9$ to $99.1$\,mm median (mean $-47.3$\,mm), whereas pure triangulation object depth improves development ($-15.0$\,mm) and confirmation ($-23.7$\,mm) splits before regressing held-out object translation ($+15.4$\,mm), motivating separate object and hand depth estimators. On the $11$-clip fresh split, the $29$-feature monotonic GBDT credibility scorer (\texttt{POSEVERIFY}) achieves $0.899$ isotonic-calibrated ($0.904$ uncalibrated raw) AUROC on clips containing both credibility classes.

\noindent\textbf{Gripper and policy evaluation protocol.}
On the $28$ EgoDex take-sides, object-bound holding frames ($54\%$) satisfy \texttt{Band A} by construction once locked; on unlocked transition frames, the gain over Ego2Robot is $+0.089$. The five-gripper pinch-point TCP convention is standardized across $14$ shared episodes. In RoboTwin~2.0~\cite{robotwin2}, matched-video conversion yields $31/52$ ($59.6\%$) on \emph{Bread in basket} versus $1/52$ ($1.9\%$) for baselines (\cref{fig:teaser}c; $22.4\%$ vs.\ $2.6\%$ in raw multi-take candidate replay). On \emph{Bread in basket} (\texttt{place\_bread\_basket}), the initial $50$-scene paired evaluation reaches $70.0\%$ for Ego2X versus $44.0\%$ zero-shot ($2.0\%$ HuRo, $4.0\%$ Ego2Robot; $52{:}17$, $p=2.9\times10^{-5}$ on the $150$ subsequent scenes). On the expanded $200$-scene paired evaluation (\cref{fig:teaser}c), Ego2X reaches $63.5\%$ (\texttt{P70}, $70$ verified episodes) and $67.0\%$ (\texttt{55 lw}, $55$ layout-weighted verified episodes; $p=0.56$ between the two Ego2X arms) versus $40.5\%$ zero-shot ($72.0\%$ with $20$ simulator expert demonstrations, $144/200$, $p=0.057$ vs.\ $70$-episode Ego2X). On \emph{Bell on scale} (\texttt{place\_object\_scale}), HuRo and Ego2Robot yield $0/53$ passing conversions and thus form no trainable policy pool. Across the $200$-scene \emph{Bell on scale} evaluation on the identical $40$ \texttt{zero-retry} verified episodes, Ego2X reaches $55.0\%$ when trained with task-aligned scene instructions and $48.0\%$ when trained with a fixed cross-task placeholder prompt inherited from the trimming script (evaluated on seen scale instructions), compared with $47.0\%$ at a half-dose budget ($20$ \texttt{zero-retry} verified episodes), $27.0\%$ with an unfiltered $40$-episode pool ($31$ \texttt{zero-retry}, $4$ retry, and $5$ failed conversions), and $17.0\%$ zero-shot. Paired scene-seed intersections span $191$ to $198$ of $200$ scenes due to simulator scene-generation retry limits.

%-------------------------------------------------------------------------
\section{Component Ablations Across Stages 2, 3, 4 and 6}
\label{sec:suppl-abl}

\begin{table}[t]
\centering
\scriptsize
\setlength{\tabcolsep}{2.0pt}
\caption{\textbf{Stage-2 depth parameterization, credibility families and closed-loop waterfall.} Top: hand depth parameterization on confirmation estimated poses ($8$ clips, $1{,}269$ slots). Middle: uncalibrated raw AUROC across multi-feature families (solo / leave-one-family-out, e.g., the $6$-feature 2D contour group vs.\ full $29$-D GBDT), complementing the isotonic-calibrated GBDT vs.\ single-feature 2D mask IoU comparison in main-paper Tab.~3. Bottom: all-slot hand $\Delta M_1$ (mm) across the five-step Stage-2 waterfall.}
\label{tab:suppl_abl2}
\begin{tabular*}{\columnwidth}{@{\extracolsep{\fill}}lrrrr@{}}
\toprule
Param.\ (Conf-8, $1{,}269$ slots) & $\Delta M_1$ & $\Delta$Ray & $\Delta$2D (px) & $\Delta M_2$ \\
\midrule
1-DoF Cauchy, $\ge 3$ inl.\ (ours) & \textbf{$-$4.13} & \textbf{$-$5.54} & \textbf{2.45} & \textbf{$-$3.22} \\
1-DoF unbounded $L_2$                & $+$32.68 & $+$28.85 & 12.52 & $+$22.09 \\
3-DoF translation Cauchy             & $+$36.30 & $+$26.45 & 24.51 & $+$25.30 \\
6-DoF $\mathrm{SE}(3)$ Kabsch        & $+$43.59 & $+$27.61 & 33.67 & $+$27.42 \\
\bottomrule
\end{tabular*}\par
\vspace{0.25em}
\begin{tabular*}{\columnwidth}{@{\extracolsep{\fill}}lcccc@{}}
\toprule
Credibility family (solo/LOFO) & LOCO & Fresh & Conf & Held \\
\midrule
Full 29-D GBDT (raw)     & \textbf{0.886} & 0.904 & \textbf{0.804} & 0.713 \\
Contour 2D (6)           & .848/.742 & \textbf{.929}/.701 & .589/.714 & .859/.623 \\
Temporal / Sym.\ (7)     & .737/.882 & .699/.908 & .696/.771 & .688/.709 \\
Multi-view reg.\ (6)     & .615/.883 & .710/.909 & .639/.804 & \textbf{.934}/.707 \\
Depth / Shape (4)        & .631/.863 & .550/.913 & .630/.769 & .431/.793 \\
Tracker internal (6)     & .539/.882 & .294/.905 & .700/.825 & .737/.725 \\
\bottomrule
\end{tabular*}\par
\vspace{0.25em}
\begin{tabular*}{\columnwidth}{@{\extracolsep{\fill}}lccc@{}}
\toprule
Closed-loop hand waterfall ($\Delta M_1$, mm) & Dev-12 & Conf-8 & Held-11 \\
\midrule
$S_1$: Raw object pose, single-frame & $+$0.08 & $-$3.32 & $-$0.18 \\
$S_2$: Hand-scaled depth fusion (circular) & $-$1.22 & $-$3.21 & $+$1.34 \\
$S_3$: Hand-ruler-free $+$ hard credibility gate & $-$1.12 & 0.00 & $-$0.13 \\
$S_4$: Hand-ruler-free, per-frame un-gated & $-$2.24 & $-$4.30 & $-$0.88 \\
$S_5$: Hand-ruler-free $+$ interval-linear (ours) & \textbf{$-$2.60} & \textbf{$-$4.31} & \textbf{$-$1.91} \\
\bottomrule
\end{tabular*}
\end{table}

\noindent\textbf{CORE and Stage-2 ablations.}
\Cref{fig:core} in the main paper illustrates occluded CORE recovery. On the $31$-clip HOT3D confirmation ladder (Fr.\ F1 / Iv@.5 / tIoU / Pt mm / Mode F1 / State), geometric proximity $G$ reaches $0.847 / 0.565 / 0.826 / 6.69 / 0.307 / 0.701$, tactile $+T$ reaches $0.920 / 0.680 / 0.897 / 3.28 / 0.189 / 0.817$, and ray anchoring $T{+}R$ reaches $0.912 / 0.690 / 0.889 / \mathbf{1.96} / 0.269 / 0.792$. Medoid bridging $T{+}R{+}B$ reaches $\mathbf{0.924} / \mathbf{0.741} / 0.915 / 11.30 / 0.379 / 0.837$, while full CORE ($T{+}R{+}B{+}E$) reaches $0.920 / 0.722 / \mathbf{0.923} / 7.82 / \mathbf{0.408} / \mathbf{0.841}$ (any-overlap interval F1 $0.727\to 0.784$). With native stage-specific (field-selective) readout, CORE reaches $\mathbf{0.924} / \mathbf{0.741} / 0.915 / 2.39 / \mathbf{0.408} / \mathbf{0.841}$ ($-4.30$\,mm $[-7.71,-0.68]$ vs.\ $G$). Across $19$ pooled estimated-pose clips (including $3$ zero-detection clips), Stage-2 contact-aligned object depth fusion (\texttt{FUSE}) over raw FoundationPose improves Fr.\ F1 by $+0.195$ $[+0.105,+0.292]$, Iv@.5 by $+0.144$ $[+0.051,+0.260]$, and median tIoU by $+0.317$ $[+0.069,+0.461]$. Pure estimated-velocity state accuracy rises from $0.076$ to $0.202$ ($+0.125$ $[+0.062,+0.200]$), while hand-ruler-free triangulation (\texttt{OW+M1lin}) lowers camera-frame contact point error over coupled fusion on the $11$-clip held-out split by $-31.1$\,mm $[-48.6,-2.6]$ ($n{=}6$ paired clips). \Cref{tab:suppl_abl2} reports Stage-2 parameterizations, feature families, and the closed-loop waterfall ($S_1$--$S_5$): circular hand-scaled fusion degrades $S_2$, single-frame gating restricts valid-slot coverage in $S_3$ ($0.0$--$9.2\%$), and un-gated triangulation ($S_4$) with interval-linear propagation ($S_5$) recovers consistent gains across all splits.

\input{tables/tab_vs_huro}
\input{tables/tab_ik_velocity}

\begin{figure}[t]
  \centering
  \includegraphics[width=0.92\columnwidth]{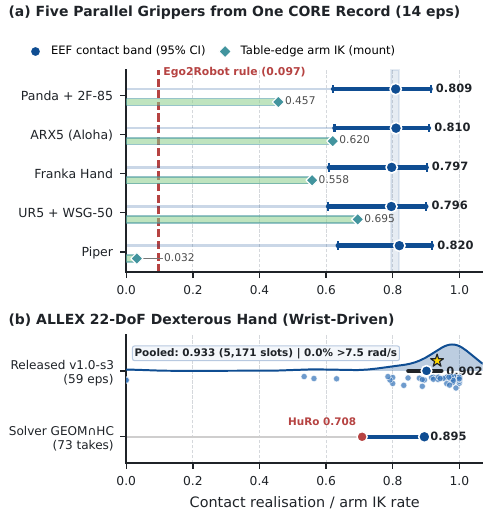}
  \caption{\textbf{Cross-embodiment compilation.} End-effector realization and arm feasibility across five parallel grippers and the compiled ALLEX dexterous hand trajectories.}
  \label{fig:embodiments}
\end{figure}

\begin{figure*}[t]
  \centering
  \includegraphics[width=0.96\textwidth]{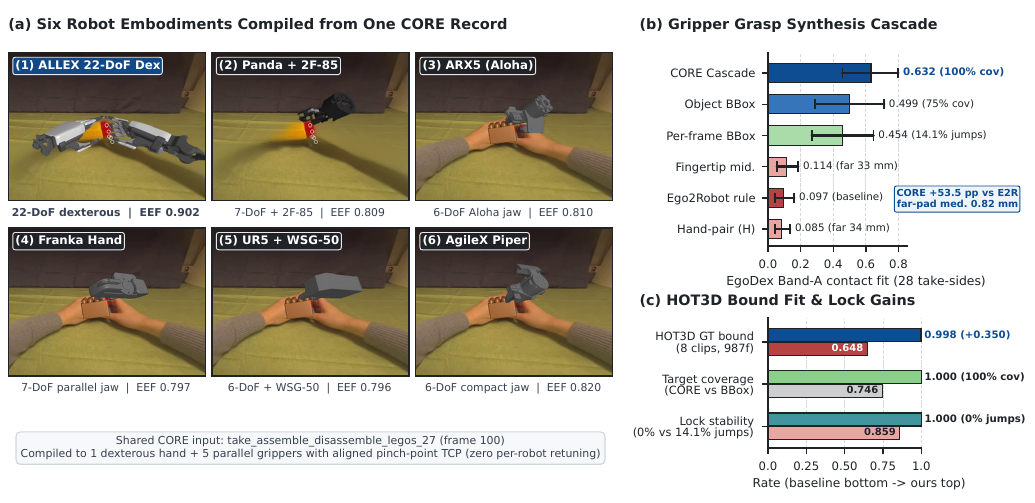}
  \caption{\textbf{Cross-embodiment compilation and parallel-gripper synthesis.} (a) One dexterous hand and five parallel grippers compiled from the identical CORE record. (b,c) Parallel-gripper synthesis cascade, HOT3D realization and interval-lock stability.}
  \label{fig:embodiments_qual}
\end{figure*}

\begin{table}[t]
\centering
\scriptsize
\setlength{\tabcolsep}{1.8pt}
\caption{\textbf{Parallel-jaw synthesis ablation} ($28$ EgoDex take-sides, $1{,}272$ trusted holding/transport frames; Near/Far: median true-mesh signed distance in mm; Jit.: TCP step in mm/frame).}
\label{tab:grip_ablation}
\begin{tabular*}{\columnwidth}{@{\extracolsep{\fill}}lcccccc@{}}
\toprule
Arm & Band A [95\% CI] & Meas. & Pen. & Near/Far & Jit. & Cov. \\
\midrule
$C_{\mathrm{full}}$ (ours)       & \textbf{0.632} [0.456, 0.799] & 0.632 & \textbf{0.063} & 0.60 / \textbf{0.82} & 7.7 & \textbf{1.00} \\
$C_{\mathrm{geom}}$ (bbox only)  & 0.499 [0.288, 0.712] & \textbf{0.669} & 0.090 & 0.50 / 3.27 & 9.7 & 0.75 \\
$C_{\mathrm{perframe}}$ (no lock)& 0.454 [0.269, 0.647] & 0.609 & 0.140 & 0.52 / 3.34 & 10.0 & 0.75 \\
$W_{\mathrm{tip}}$ (fingertips)  & 0.114 [0.054, 0.185] & 0.114 & 0.213 & 8.88 / 32.6 & 8.5 & 1.00 \\
$H_{\mathrm{handpair}}$ (hand)   & 0.085 [0.043, 0.136] & 0.085 & 0.241 & 7.89 / 34.0 & 7.6 & 1.00 \\
$W_{\mathrm{wrist}}$ (wrist)     & 0.006 [0.000, 0.013] & 0.006 & 0.121 & 24.0 / 90.3 & \textbf{7.2} & 1.00 \\
\bottomrule
\end{tabular*}
\end{table}

\noindent\textbf{Dexterous IK, retiming and gripper synthesis.}
On HOT3D ($31$ clips, $72$ pairs), removing mode pools or normal alignment yields $6.62$\,mm ($0.973$ band) and $6.82$\,mm ($0.968$ band) versus $6.78$\,mm ($0.969$ band) for full \texttt{CARD} (Eq.~\ref{eq:ik}), while on noisy monocular hand predictions ($73$ groups) \texttt{CARD} achieves $0.861$ band ($7.86$\,mm) with oracle contacts and $0.379$ ($32.11$\,mm) with estimated contacts versus $0.268$ ($35.84$\,mm) for wrist following (\texttt{wf}). Across EgoDex $\texttt{GEOM}{\cap}\texttt{HC}$ ($3{,}723$ frames), pseudo-signed frame penetration ($<-1$\,mm on non-watertight meshes) is $4.43\%$ for Ego2X versus $4.06\%$ for HuRo ($p=0.393$, \cref{tab:vs_huro}). At an equalized 22-joint caliber (\cref{tab:ik_velocity}), our step limiter bounds all frames at $\le 7.5$\,rad/s ($0.0\%$ true excursions across rate-retimed ALLEX trajectories), whereas HuRo reaches $63.92$\,rad/s (\cref{fig:ikdex,fig:embodiments,fig:embodiments_qual}). \Cref{tab:grip_ablation} reports the six-arm parallel-gripper decomposition.

\input{tables/tab_conversion}

\begin{table}[t]
\centering
\scriptsize
\setlength{\tabcolsep}{1.6pt}
\caption{\textbf{CORE-field and compiler ablations on \emph{Bell on scale} (\texttt{place\_object\_scale})} ($53$ specifications across $24$ takes; \texttt{0-retry}: \texttt{zero-retry} episodes passing on the first attempt without planner retry; Holm-adjusted exact McNemar $p$ vs.\ full Ego2X). $^{\dagger}$Unsnapped fingertip midpoint ($p=2.0{\times}10^{-11}$ vs.\ centroid-clamped).}
\label{tab:suppl_abl4}
\begin{tabular*}{\columnwidth}{@{\extracolsep{\fill}}lcccccc@{}}
\toprule
Arm & Succ & 0-retry & Miss & Place & Plan & Holm $p$ \\
\midrule
HuRo / Ego2Robot            & 0/0 & 0/0 & 53/52 & 0/1 & 0/0 & $4.8{\times}10^{-7}$ \\
Ego2X (full)                & \textbf{45} & \textbf{40} & 1 & 5 & 2 & ref. \\
w/o binding $\mathbf{T}_{OG}$ & 0$^{*}$ & 0 & 1 & 50 & 2 & $3.4{\times}10^{-13}$ \\
w/o anchors, clamped        & \textbf{48} & \textbf{41} & 1 & 2 & 2 & 0.51 \\
w/o anchors, unsnapped$^{\dagger}$ & 8 & 4 & 37 & 6 & 2 & $7.3{\times}10^{-11}$ \\
w/o CORE state bounds       & 39 & 36 & 1 & 3 & 10 & 0.44 \\
w/o 6-roll, w/o live retry  & 41/41 & 40/39 & 5/6 & 4/5 & 3/1 & 0.44 \\
\bottomrule
\end{tabular*}
\\[0.15em]{\scriptsize $^{*}$Lifts the object on $52/53$ episodes before failing placement ($84.9\%$ full, $90.6\%$ clamped).}
\end{table}

\noindent\textbf{Simulation conversion and VLA ablations.}
\Cref{tab:conversion,tab:suppl_abl4} detail closed-loop conversion yields and failure modes. On \emph{Bell on scale} (\texttt{place\_object\_scale}), removing object-frame transport binding $\mathbf{T}_{OG}$ lifts the object on $52/53$ runs yet fails placement on $50/53$ ($0/53$ task success), whereas comparing \texttt{centroid clamping} against unsnapped anchor-free grasps ($48/53$ vs.\ $8/53$, McNemar $41{:}1$, $p=2.0\times 10^{-11}$) isolates the contribution of clamping antipodal grasp midpoints toward the object support-hull centroid. Under worst-case imputation of all unpaired RoboTwin scene seeds ($2$--$7$ of $200$), all primary VLA comparisons hold: full Ego2X vs.\ zero-shot ($p\le 5.3\times 10^{-8}$), unfiltered $40$-episode pool vs.\ \texttt{zero-retry} verified Ego2X ($p\le 1.3\times 10^{-4}$), half-dose $20$-episode Ego2X vs.\ zero-shot ($p\le 3.2\times 10^{-6}$), and task-aligned scene instructions vs.\ zero-shot ($p\le 1.2\times 10^{-8}$).

%-------------------------------------------------------------------------
\section{Implementation Details and Measured Runtimes}
\label{sec:suppl-impl}

\noindent\textbf{Stack and hyperparameters.}
Stage~1 runs monocular EgoHand~\cite{egohand} with projection fill (ACE-Ego-Hand~\cite{aceegohand} for 2D boxes only), EgoHOS-seeded~\cite{egohos} SAM~3~\cite{sam3} video tracking with an occlusion watchdog and VLM verification, SAM~3D~\cite{sam3d}, FoundationPose~\cite{foundationpose}, MoGe~3~\cite{moge}, and monocular SLAM at $960\times 540$ virtual intrinsics. Stage~2 runs the $29$-feature monotonic GBDT credibility scorer (\texttt{POSEVERIFY}; maximum depth $3$, minimum leaf $50$, $200$ trees, learning rate $0.05$), contact-aligned object depth fusion (\texttt{FUSE}), and $15$\,mm-parallax-gated hand depth refinement (\texttt{OW+M1lin}) with $15$-frame inner-edge linear interval propagation. Stage~4 enforces a $7.5$\,rad/s joint-rate bound matching Eq.~\ref{eq:ik}. Stage~6 fine-tunes X-VLA~\cite{xvla} with LoRA ($r{=}8$, $\alpha{=}16$, bf16, batch $4\times 4$, learning rate $10^{-4}$, $3{,}000$ steps, $300$-step freeze, $600$-step warmup).

\noindent\textbf{Hardware and measured wall-clock times.}
All conversion stages execute locally on an $8\times\text{NVIDIA RTX 4090}$ ($24$\,GB) workstation, with X-VLA fine-tuning on one NVIDIA A100-80GB GPU. Across the $220$-take EgoDex conversion batch (\cref{tab:suppl_stage_times}), a completed take requires a median of $94.0$\,min ($5{,}642$\,s over $74$ completed takes; $86.2$\,min over all $220$ takes including early stops), dominated by multi-hypothesis pose refinement ($2{,}707$\,s median; $59.5$--$13{,}468$\,s across $74$ completed runs) and monocular hand estimation ($875$\,s); maxima reflect local GPU queue contention. Stage-2 depth fusion and credibility scoring add $27.3$--$240.7$\,s per clip. Single-A100 X-VLA fine-tuning ($3{,}000$ steps, $47.5$\,MB LoRA adapter) takes $187.2$, $179.0$, and $138.5$\,min for $70$, $30$, and $10$ episodes.

\begin{table}[t]
\centering
\scriptsize
\setlength{\tabcolsep}{3.5pt}
\caption{\textbf{Measured per-stage wall-clock runtime per take (seconds)} across the $220$-take EgoDex conversion batch (including early-stopped runs) on an $8\times\text{RTX 4090}$ workstation.}
\label{tab:suppl_stage_times}
\begin{tabular*}{\columnwidth}{@{\extracolsep{\fill}}lrrrr@{}}
\toprule
Stage & $n$ & Min & Median & Max \\
\midrule
Pose refine & 122 & 4.3 & 2707.3 & 14629.8 \\
Monocular hand~\cite{egohand} & 220 & 90.1 & 874.6 & 3527.8 \\
Object pose~\cite{foundationpose} & 121 & 58.8 & 444.4 & 7201.5 \\
World align & 120 & 87.6 & 400.5 & 3199.2 \\
Object recon~\cite{sam3d} & 196 & 16.7 & 333.9 & 43003.1 \\
Object pick & 164 & 35.7 & 178.6 & 17875.7 \\
Arm erase~\cite{sam3} & 204 & 30.8 & 137.9 & 4739.7 \\
Depth~\cite{moge2} & 199 & 14.7 & 120.1 & 1359.2 \\
MANO fit~\cite{mano} & 209 & 44.9 & 102.6 & 734.4 \\
Camera track (SLAM) & 219 & 25.1 & 81.9 & 810.4 \\
Hand-object seed~\cite{egohos} & 201 & 7.4 & 78.8 & 1589.4 \\
Mask watchdog~\cite{sam3} & 200 & 5.4 & 76.8 & 19369.4 \\
Contact depth refinement & 74 & 5.0 & 44.2 & 516.9 \\
Render & 88 & 0.5 & 43.3 & 373.0 \\
Contact semantics~\cite{egotac} & 209 & 17.4 & 32.7 & 273.3 \\
Segmentation QA (VLM) & 199 & 5.6 & 23.0 & 144.8 \\
Contact synthesis \& IK (Stages 3--5) & 74--209 & 0.2 & 0.4--12.3 & 97.5 \\
\bottomrule
\end{tabular*}
\end{table}
